# Supplementary material for: Pressure-induced electronic and structural evolution of EuIrGe3
Source: arXiv:2609.20376 source file (2026-09-17)
Supplement: Supplementary file 1 [file EuIrGe3_SM.tex]

\documentclass[aps,prx,onecolumn,10pt,superscriptaddress,showpacs,showkeys]{revtex4-1}
\usepackage{subcaption}
\usepackage{amsmath,latexsym,amsfonts,amssymb}
\usepackage{natbib}
\usepackage{epsfig}
\usepackage{graphicx}
\usepackage{inputenc}
\usepackage{setspace}
\usepackage{multirow}
\usepackage{array}
\usepackage{tabularx}
\usepackage{bm}
\usepackage{color}
\usepackage{xcolor}
\usepackage{gensymb}
\usepackage[left]{lineno}
\usepackage{float} 
\usepackage{ulem}
\usepackage{siunitx}
%\usepackage{booktabs}

\newcommand{\yu}{\textcolor{red}}

\date{\today}
\begin{document}


\title{Supplement material : Pressure-induced electronic and structural evolution of EuIrGe$_3$}

\author{N. S. Dhami}
\email{naveen-singh.dhami@synchrotron-soleil.fr}
\affiliation{Institute of Physics, Bijeni\v{c}ka cesta 46, 10000, Zagreb, Croatia}
\affiliation{Synchrotron SOLEIL, L’Orme des Merisiers, Saint Aubin BP 48, 91192 Gif-sur-Yvette, France}

\author{V. Balédent}
\affiliation{Université Paris-Saclay, CNRS, Laboratoire de Physique des Solides, UMR-8502, 91405, Orsay, France}
\affiliation{Institut universitaire de France (IUF), Paris, France}

\author{ I. Batistić}
\affiliation{Department of Physics, Faculty of Science, University of Zagreb, Bijeni\v{c}ka 32, 10000 Zagreb, Croatia}


\author{C. M. N. Kumar}
\affiliation{The Henryk Niewodniczański, Institute of Nuclear Physics, Polish Academy of Sciences, ul. Radzikowskiego 152, 31-342 Kraków, Poland}


\author{D. Kaczorowski}
\affiliation{Institute of Low Temperature and Structure Research, Polish Academy of Sciences, Okólna 2, 50-422 Wrocław, Poland}

\author{L. Nataf}
\affiliation{Synchrotron SOLEIL, L’Orme des Merisiers, Saint Aubin BP 48, 91192 Gif-sur-Yvette, France}


\author{J. M. Ablett}
\affiliation{Synchrotron SOLEIL, L’Orme des Merisiers, Saint Aubin BP 48, 91192 Gif-sur-Yvette, France}

\author{J.-P. Rueff}
\affiliation{Synchrotron SOLEIL, L’Orme des Merisiers, Saint Aubin BP 48, 91192 Gif-sur-Yvette, France}
\affiliation{Laboratoire de Chimie Physique-Matière et Rayonnement, Sorbonne Université, CNRS, 75005 Paris, France}

\author{J. P. Itié}
\affiliation{Synchrotron SOLEIL, L’Orme des Merisiers, Saint Aubin BP 48, 91192 Gif-sur-Yvette, France}

\author{P. Fertey}
\affiliation{Synchrotron SOLEIL, L’Orme des Merisiers, Saint Aubin BP 48, 91192 Gif-sur-Yvette, France}

\author{S. R. Shieh}
\affiliation{Department of Earth Sciences, Department of Physics and Astronomy, University of Western Ontario, London, Ontario N6A-5B7, Canada}

\author{P. Popčević}
\affiliation{Institute of Physics, Bijeni\v{c}ka cesta 46, 10000, Zagreb, Croatia}

\author{Y. Utsumi Boucher}
\email{yutsumi@ifs.hr}
\affiliation{Institute of Physics, Bijeni\v{c}ka cesta 46, 10000, Zagreb, Croatia}


\maketitle

\section{Powder X-ray diffraction}








\begin{figure*}[!htb]
    \centering
    \includegraphics[width=1.0\textwidth]{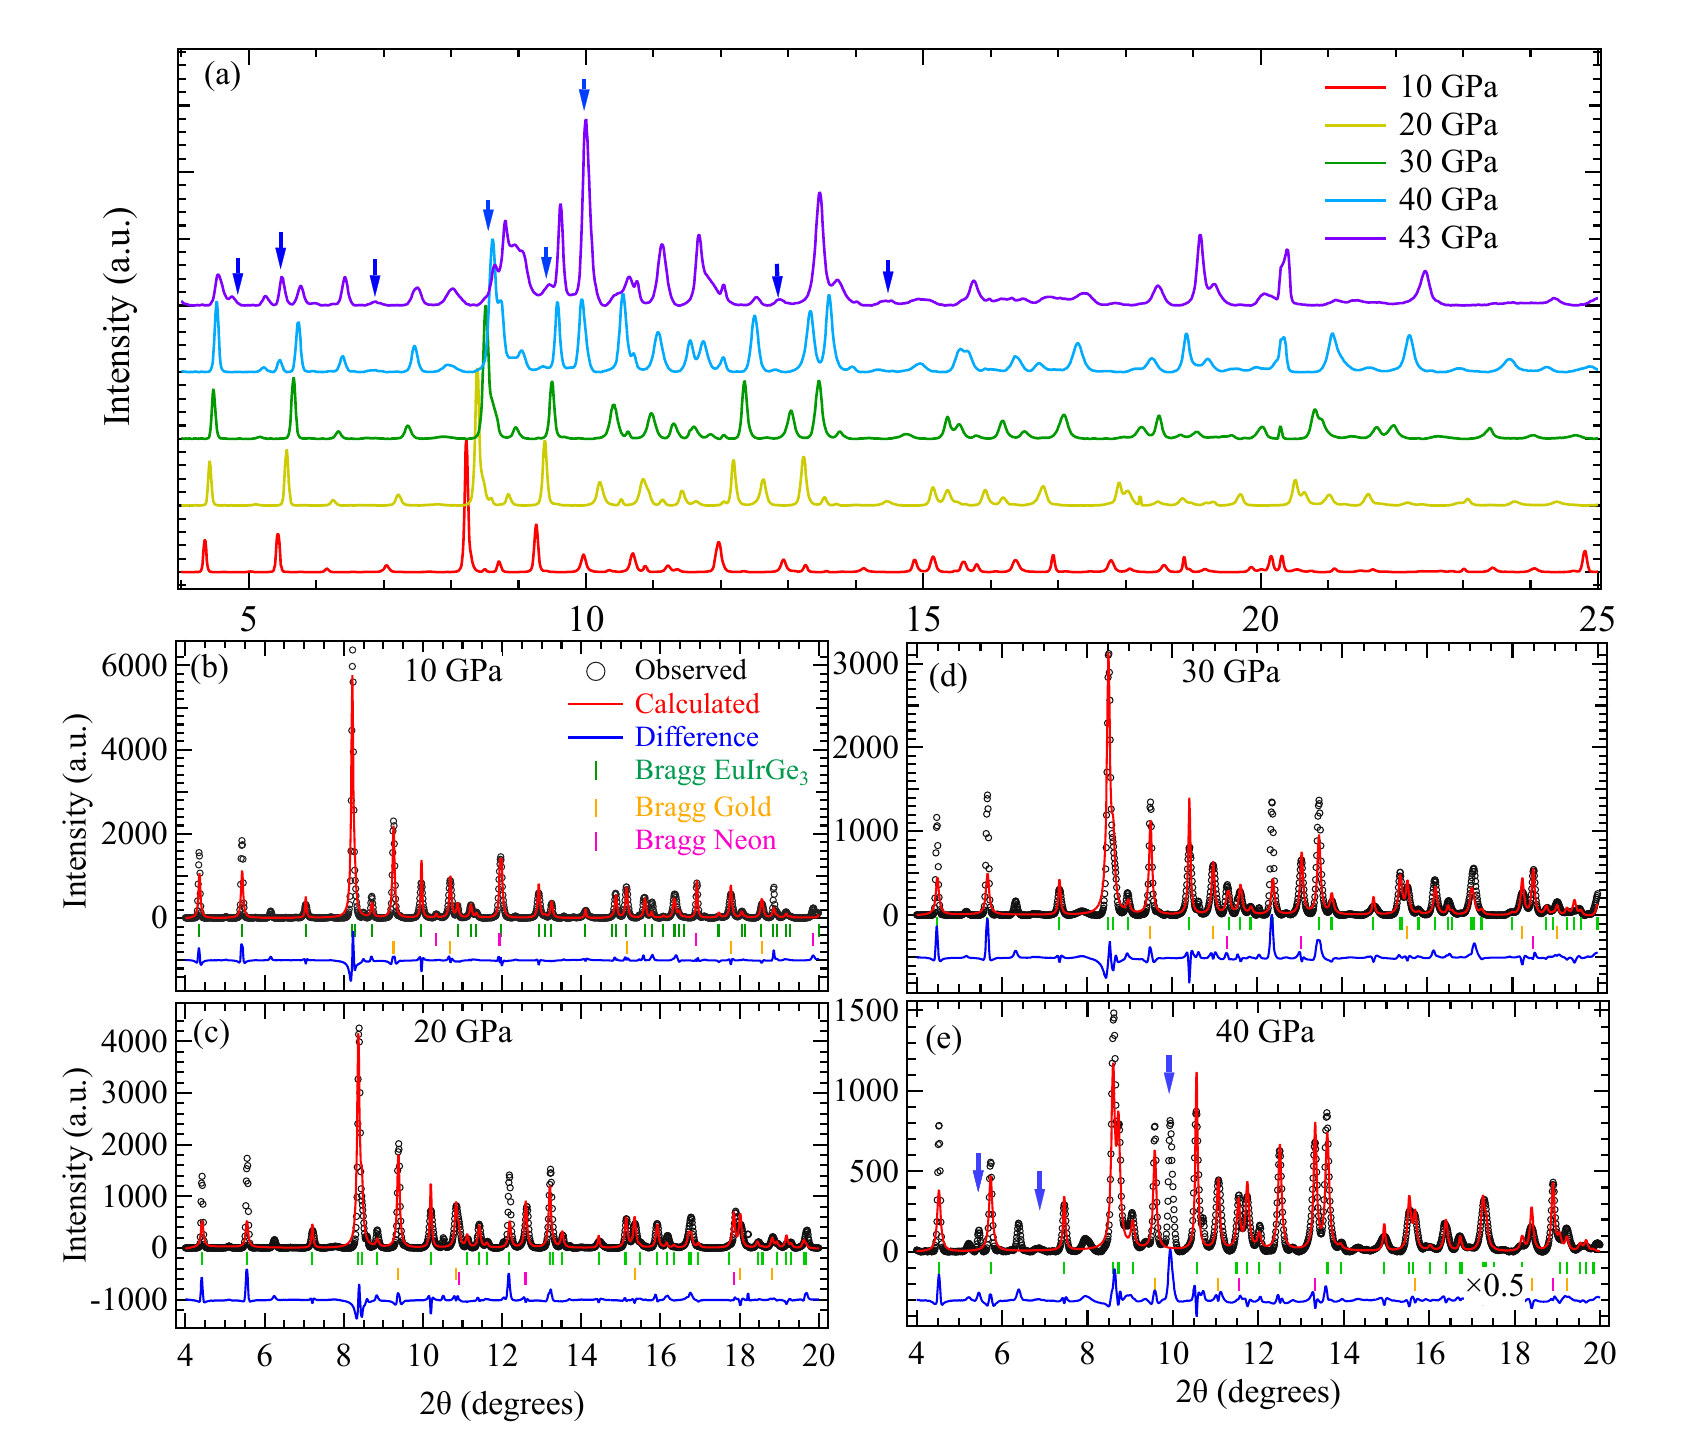}
    \caption{ (a) Synchrotron powder XRD patterns of EuIrGe$_3$ at selected pressures, with blue arrows indicating the emergence of new diffraction peaks at higher pressure. The corresponding  Rietveld refinement at (b) 10 GPa, (c) 20 GPa, (d) 30 GPa, and (e) 40 GPa. The vertical bars indicate the calculated Bragg peak positions of EuIrGe$_3$ (green), gold (orange), and neon (magenta).}
    \label{figAP2}
\end{figure*}


\begin{table}[htbp]
\centering

\begin{tabular}{c c c c c c c}
\hline\hline
$P$ (GPa) &
$z_{\rm Ge2}$ &
$z_{\rm Ge1}$ &
$z_{\rm Ir}$ &
$R_{\rm wp}$ &
$R_{\rm exp}$ &
$\chi^2$ \\
\hline
10 & 0.5817(25) & 0.2420(22) & 0.3507(11) & 32.51 & 9.49 & 11.73 \\
20 & 0.5606(22) & 0.2442(14) & 0.3557(14) & 39.71 & 9.16 & 18.79 \\
30 & 0.5375(21) & 0.2217(15) & 0.3559(11) & 40.97 & 9.31 & 19.36 \\
40 & 0.5320(26) & 0.2118(16) & 0.3498(19) & 40.10 & 9.9 & 16.40 \\
\hline\hline
\end{tabular}
\caption{Atomic positions and Rietveld refinement parameters of EuIrGe$_3$ (space group $I4mm$, No.~107) at room temperature under pressure. Eu occupies the $2a$ Wyckoff site at $(0,0,0)$; Ge2 and Ir occupy the $2a$ sites at $(0,0,z)$, and
Ge1 occupies the $4b$ site at $(0,\tfrac12,z)$. Structural parameters and
refinement results are given for pressures of 10--40~GPa. $R_{\mathrm{wp}}$, $R_{\mathrm{exp}}$, and $\chi^2$ denote the weighted-profile residual, expected residual, and goodness-of-fit statistic, respectively.}
\label{tab:EuIrGe3_refinement}
\end{table}

\newpage


\section{Resistivity data analysis}	




  
%\appendix

%\section{Resistivity data analysis}















%\begin{table*}[h]
%\centering
%\footnotesize

%\vspace{8pt}
%\textbf{ Bloch--Gr\"uneisen (BG) Fit} \quad
%$\rho(T)=\rho_0 + A_{\rm BG}\left(\frac{T}{\Theta_R}\right)^5
%\int_{0}^{\Theta_R/T}
%\frac{x^5 e^{x}}{\left(e^{x}-1\right)^2}dx$\\
%[2pt]

%\begin{tabular}{cccc|cccc}
%\hline
%\multicolumn{4}{c|}{Run1} & \multicolumn{4}{c}{Run2} \\
%\hline
%$P$ (GPa) &
%$\rho_0$ ($\mu\Omega$cm) &
%$A_{\rm BG}$ ($\mu\Omega$cm) &
%$\Theta_R$ (K) &
%$P$ (GPa) &
%$\rho_0$ ($\mu\Omega$cm) &
%$A_{\rm BG}$ ($\mu\Omega$cm) &
%$\Theta_R$ (K) \\
%\hline
%0.00  & 8.996(35)  & $4.944(53)\times10^{1}$ & 287.4(3.1) &
%0.00  & 5.492(56)  & $4.405(74)\times10^{1}$ & 264.5(4.7) \\

%3.00  & 10.406(87) & $5.716(11)\times10^{1}$ & 296.7(5.9) &
%5.00  & 10.161(73) & $5.679(9)\times10^{1}$  & 299.3(4.8) \\

%6.00  & 11.537(87) & $5.465(11)\times10^{1}$ & 307.6(6.5) &
%8.00  & 19.919(75) & $6.621(9)\times10^{1}$  & 295.8(4.2) \\

%9.00  & 21.759(115) & $6.710(14)\times10^{1}$ & 333.9(7.4) &
%12.00 & 32.309(85) & $7.477(12)\times10^{1}$ & 313.9(5.2) \\

%10.00 & 25.701(101) & $6.834(13)\times10^{1}$ & 344.9(7.1) &
%15.00 & 52.177(230) & $9.260(33)\times10^{1}$ & 370.3(13.5) \\

%13.00 & 30.670(112) & $7.092(16)\times10^{1}$ & 365.5(8.3) &
%18.00 & 57.943(267) & $9.854(37)\times10^{1}$ & 376.4(14.6) \\

%15.00 & 36.342(107) & $7.594(17)\times10^{1}$ & 402.4(8.7) &
%&             &                         &             \\
%\hline
%\end{tabular}

%\caption{Fitting parameters obtained from the BG model applied to the temperature-dependent electrical resistivity of EuIrGe$_3$ measured during Run1 and Run2 as a function of pressure. The BG fits were performed over the temperature range 50--300~K for higher pressure and 15-300 K for ambient pressure.}
%\label{tab:Res_fit}
%\end{table*}    


\begin{table*}[h]
\centering
\footnotesize

\vspace{8pt}
\textbf{Bloch--Gr\"uneisen (BG) Fit} \quad
$\rho(T)=\rho_0 + A_{\rm BG}\left(\frac{T}{\Theta_R}\right)^5
\int_{0}^{\Theta_R/T}
\frac{x^5 e^{x}}{\left(e^{x}-1\right)^2}dx$\\[2pt]

\begin{tabular}{cccc|cccc}
\hline
\multicolumn{4}{c|}{Run1} & \multicolumn{4}{c}{Run2} \\
\hline
$P$ (GPa) &
$\rho_0$ ($\mu\Omega$cm) &
$A_{\rm BG}$ ($\mu\Omega$cm) &
$\Theta_R$ (K) &
$P$ (GPa) &
$\rho_0$ ($\mu\Omega$cm) &
$A_{\rm BG}$ ($\mu\Omega$cm) &
$\Theta_R$ (K) \\
\hline
0.00  & 9.00(4)  & 49.4(5) & 287.4(3) &
0.00  & 5.49(6)  & 44.1(7) & 264.5(5) \\

3.00  & 10.41(9) & 57.16(11) & 296.7(6) &
5.00  & 10.16(7) & 56.79(9)  & 299.3(5) \\

6.00  & 11.54(9) & 54.65(11) & 307.6(7) &
8.00  & 19.92(8) & 66.21(9)  & 295.8(4) \\

9.00  & 21.76(12) & 67.10(14) & 333.9(7) &
12.00 & 32.31(9)  & 74.77(12) & 313.9(5) \\

10.00 & 25.70(10) & 68.34(13) & 344.9(7) &
15.00 & 52.2(4) & 92.6(3) & 370.3(14) \\

13.00 & 30.67(11) & 70.92(16) & 365.5(8) &
18.00 & 57.9(3) & 98.5(3) & 376.4(15) \\

15.00 & 36.34(11) & 75.94(17) & 402.4(9) &
& & & \\
\hline
\end{tabular}

\caption{Fitting parameters obtained from the BG model applied to the
temperature-dependent electrical resistivity of EuIrGe$_3$ measured during
Run1 and Run2 as a function of pressure. The BG fits were performed over
the temperature range 50--300~K for higher pressures and 15--300~K at
ambient pressure.}
\label{tab:Res_fit}
\end{table*}




%\begin{figure*}[!htb]
 %   \centering
    %\includegraphics[width=1.0\textwidth]{Supporting_material/EIG_DOS_P.png}
    %\caption{Pressure dependence of the partial density of states (PDOS) of EuIrGe$_3$. The Ge1-$4s$, Ge2-$4s$, and Ir-$5d$ states exhibit pronounced changes near the Fermi energy with increasing pressure, whereas the contributions from the other orbitals remain comparatively unchanged.}
    %\label{fig1}
%\end{figure*}



%\bibliographystyle{apsrev}
%\bibliography{SM_EuIrGe3}




\end{document}
